# Supplementary material for: GDI: Rethinking What Makes Reinforcement Learning Different From Supervised Learning
Source: arXiv:2106.06232 source file (2022-01-09)

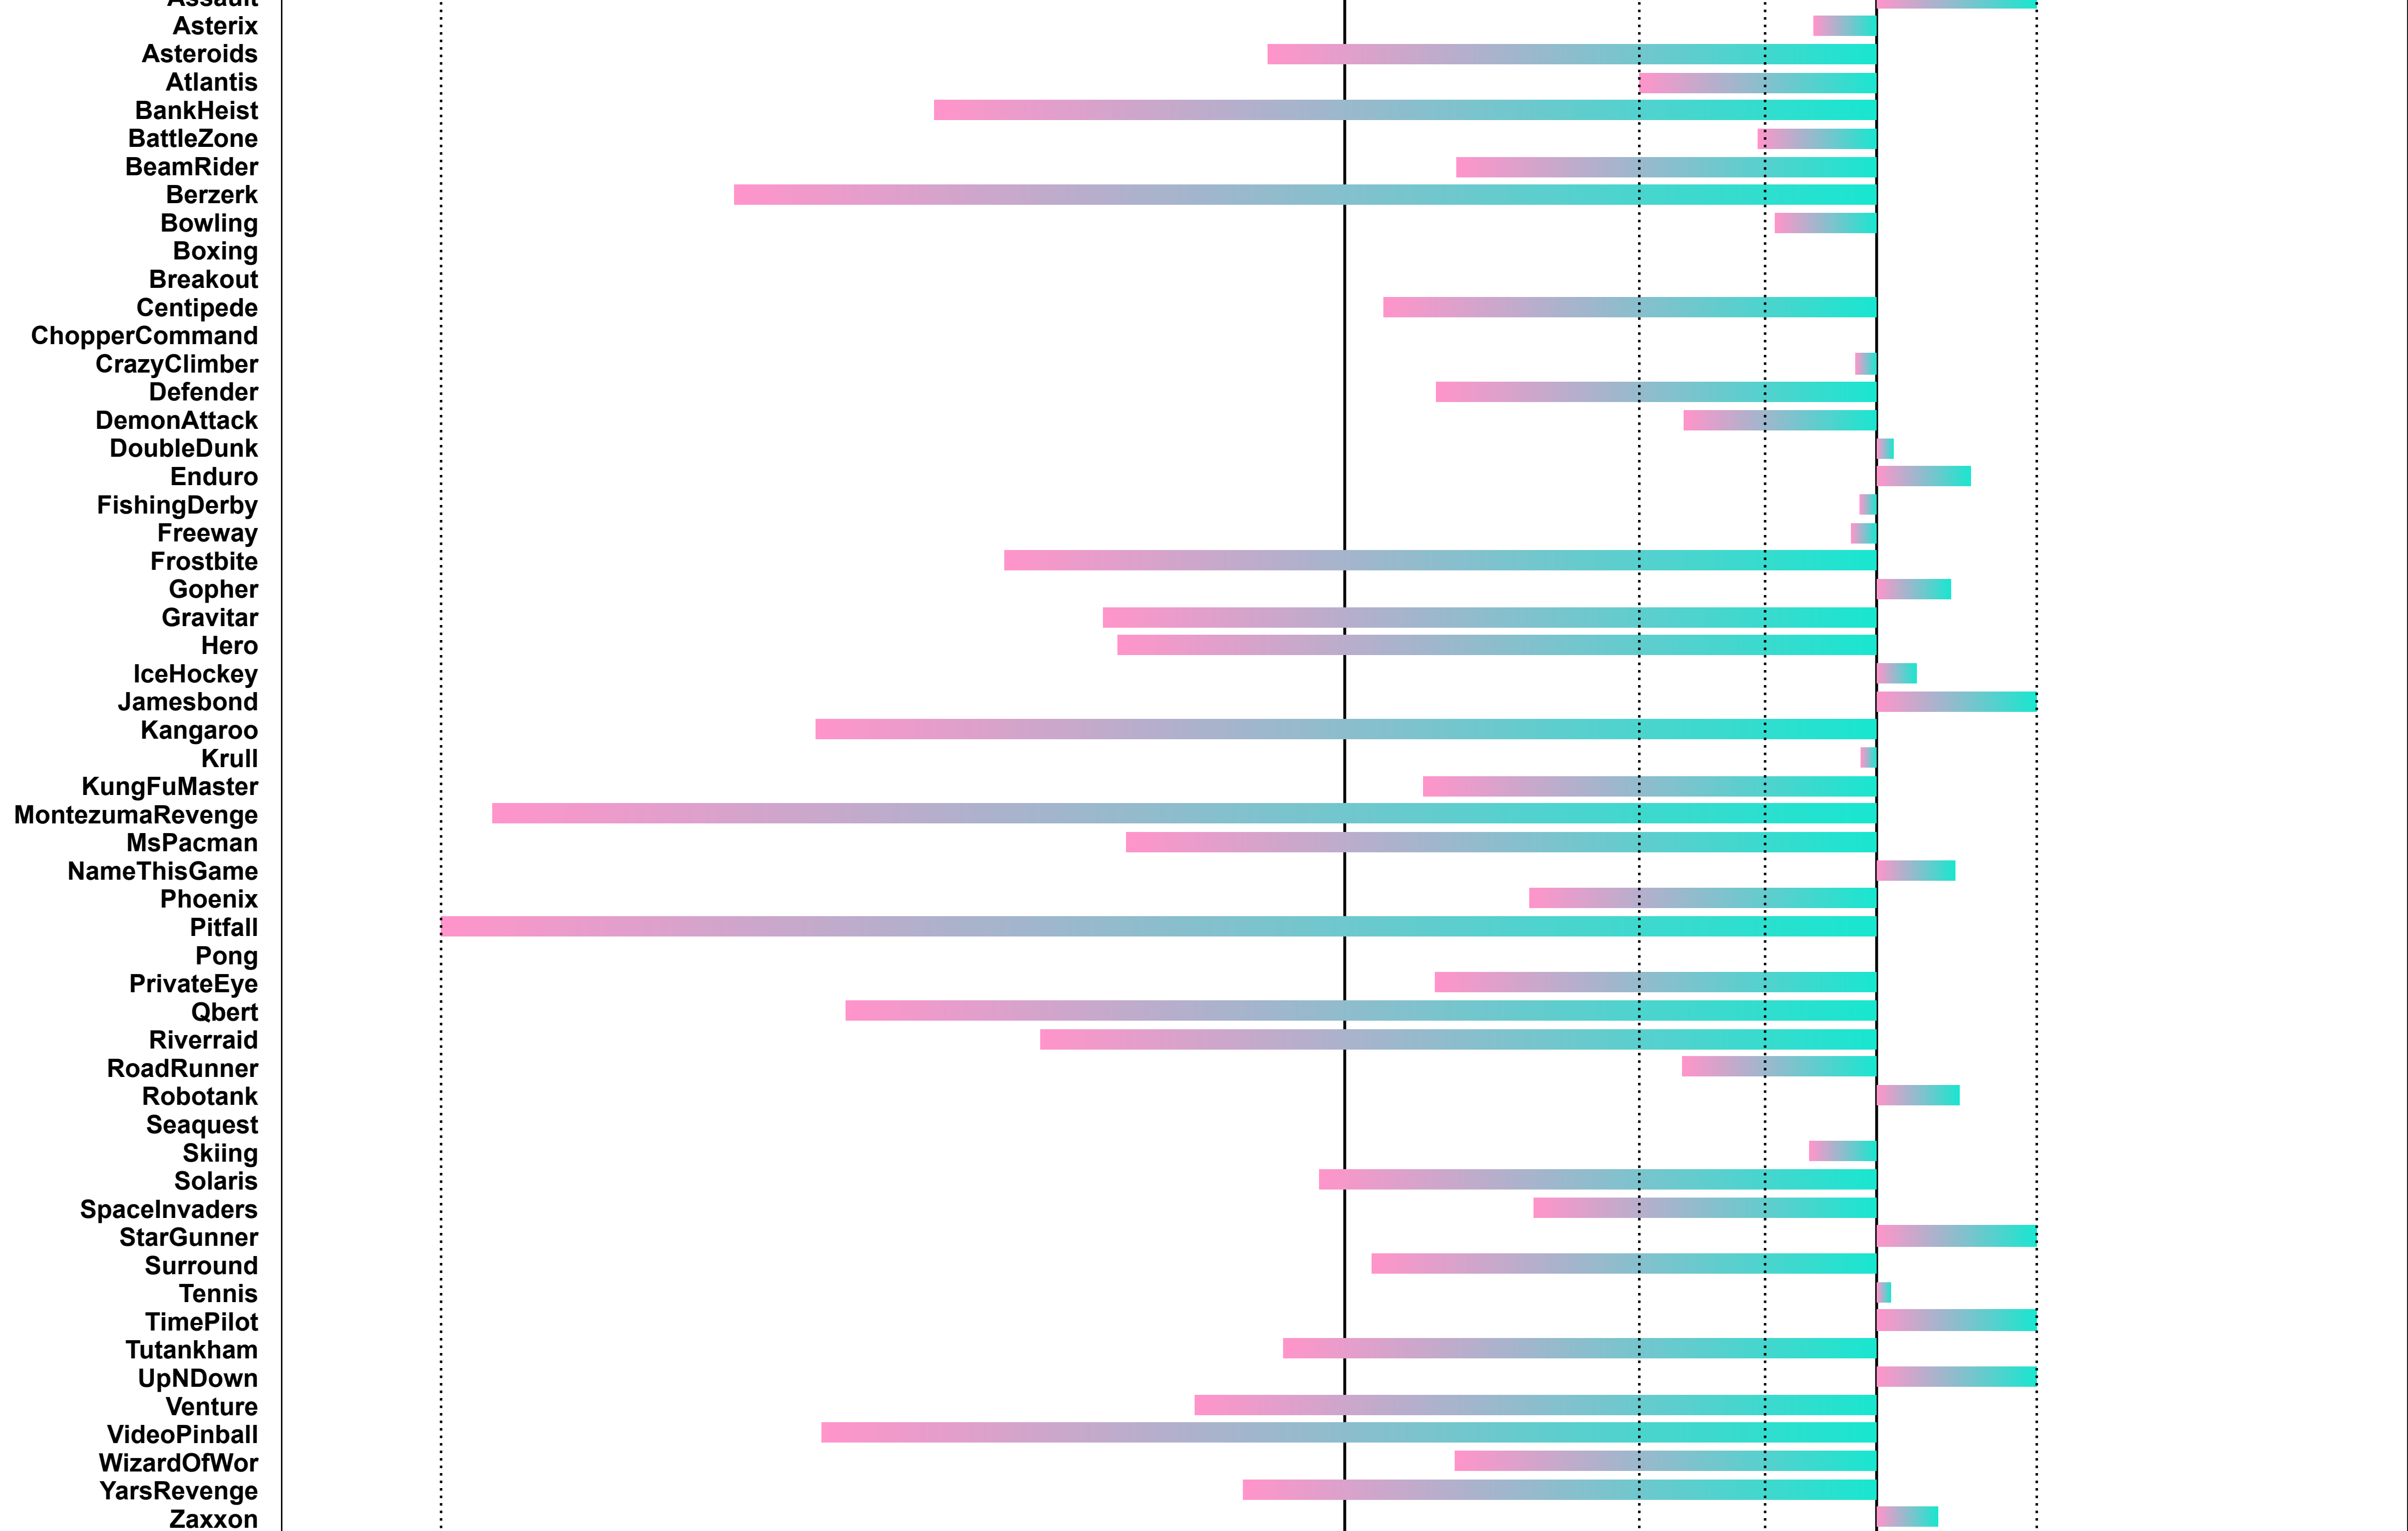

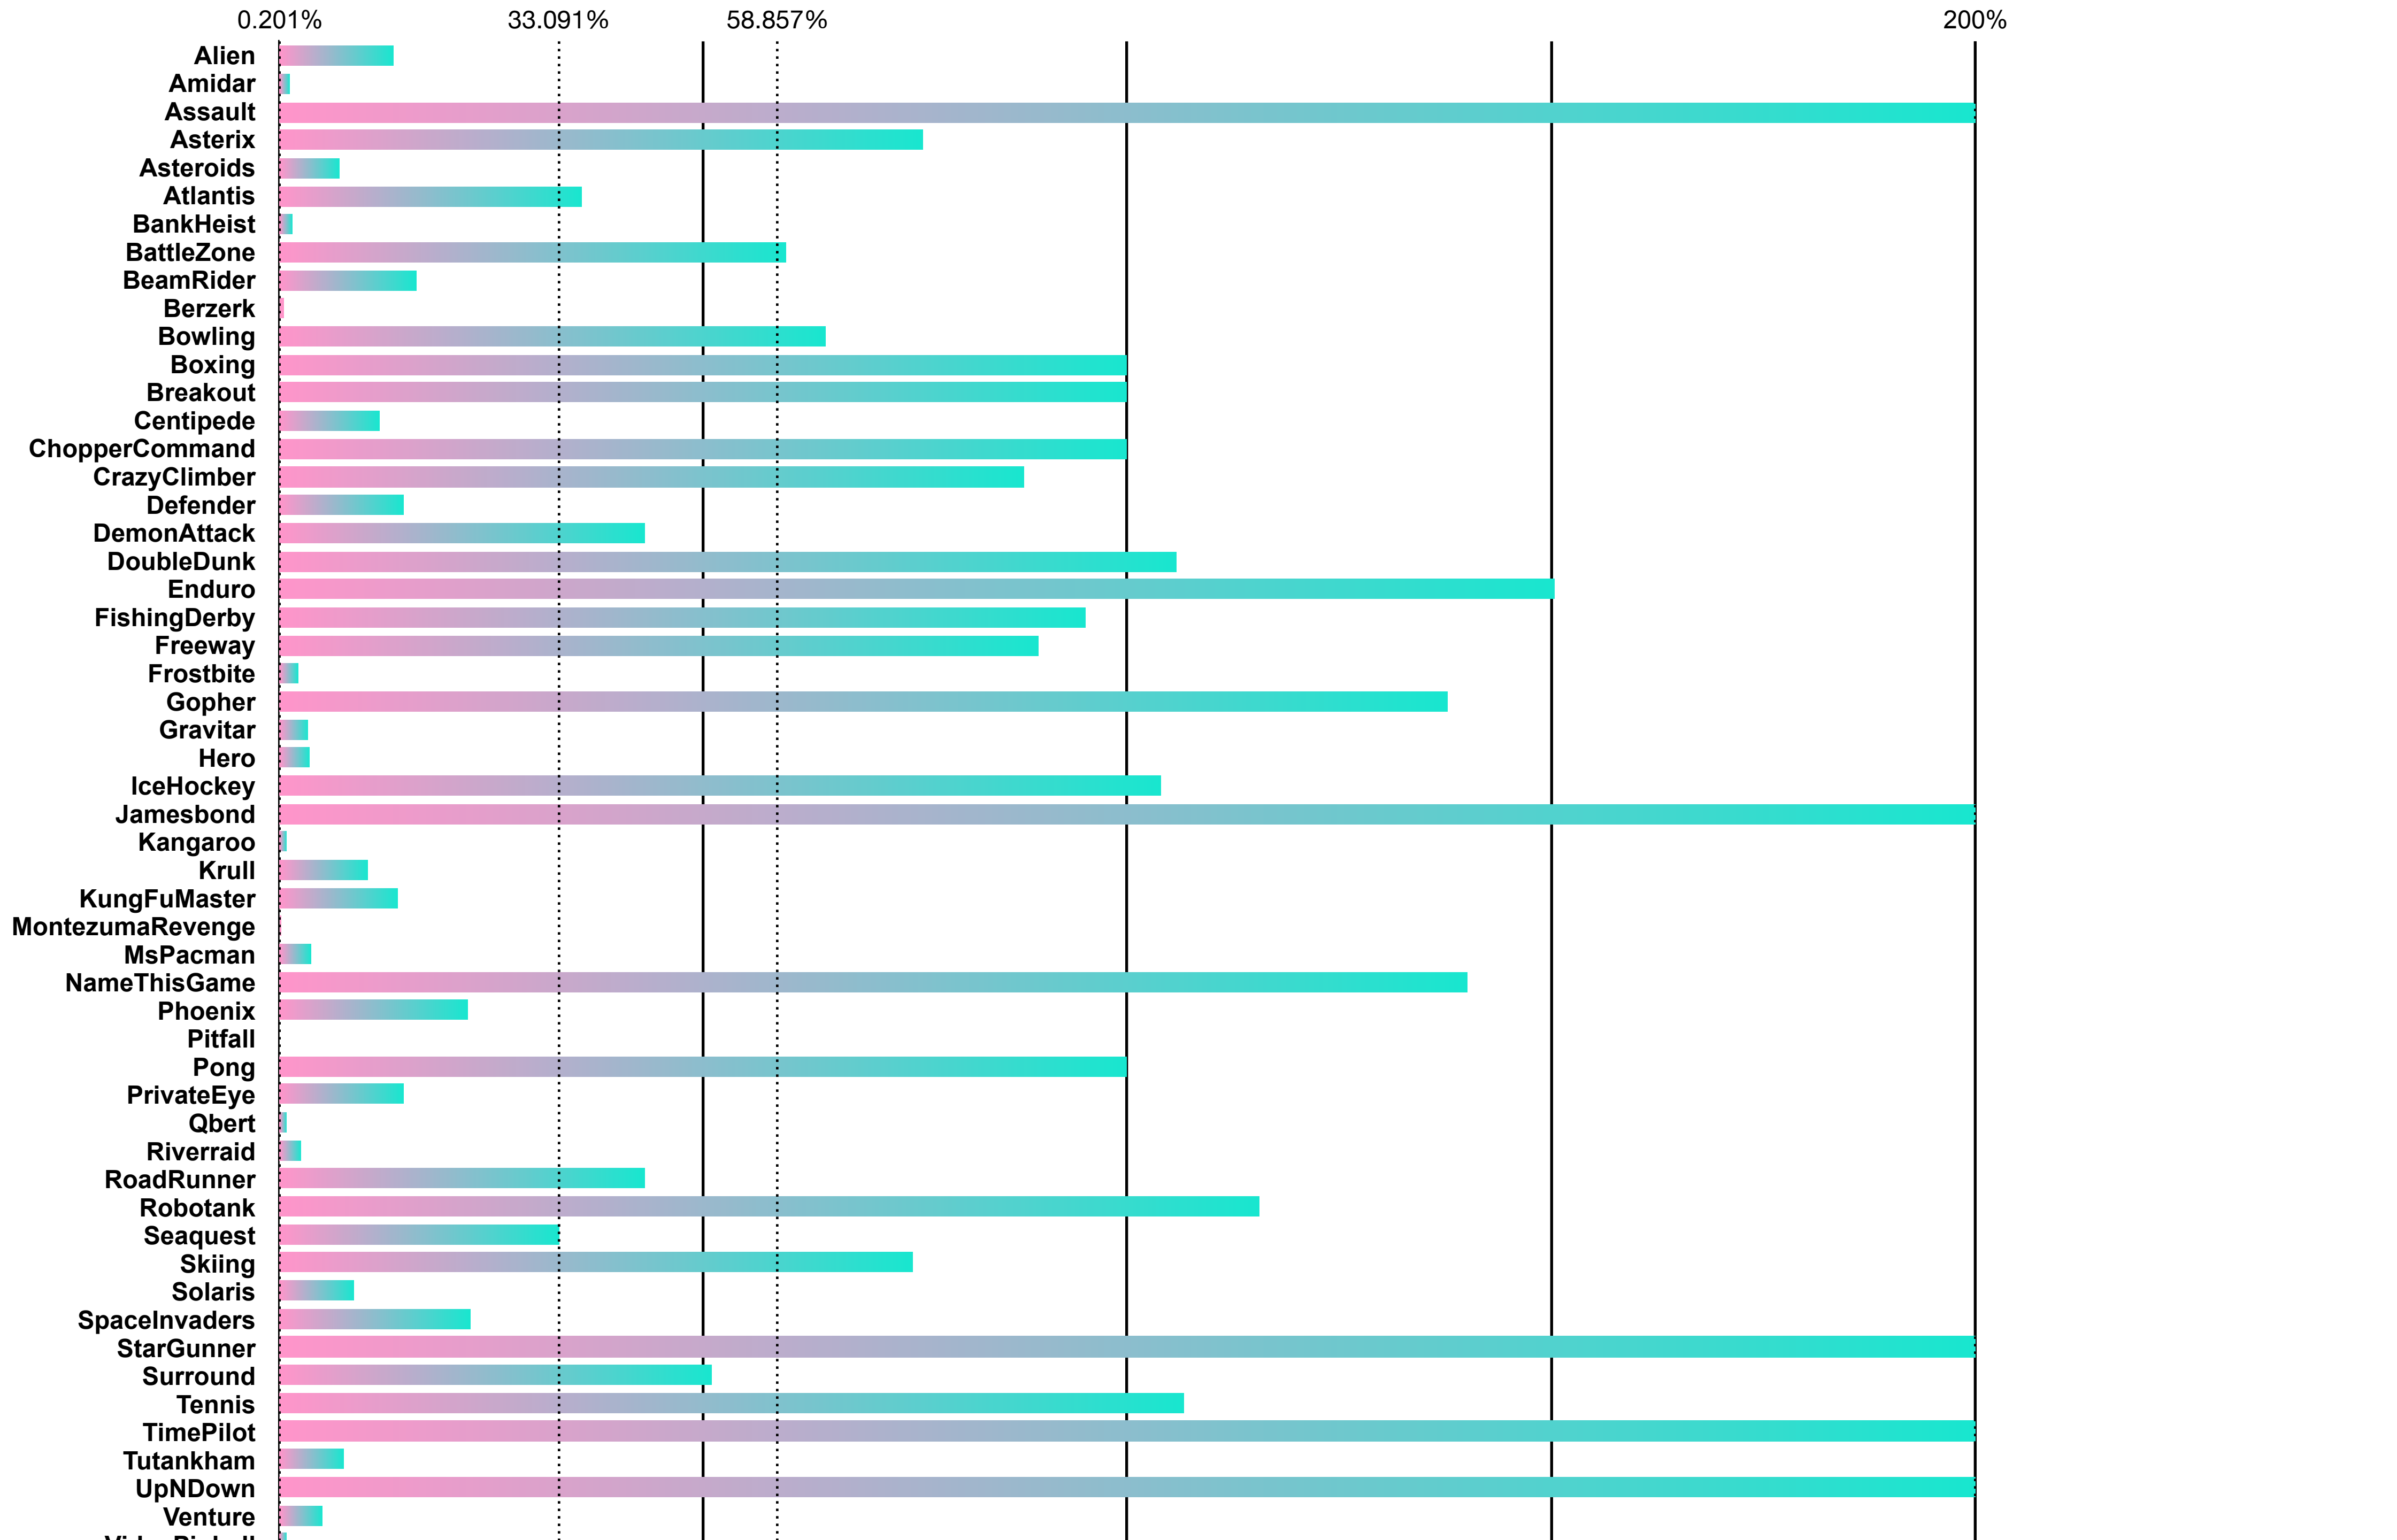

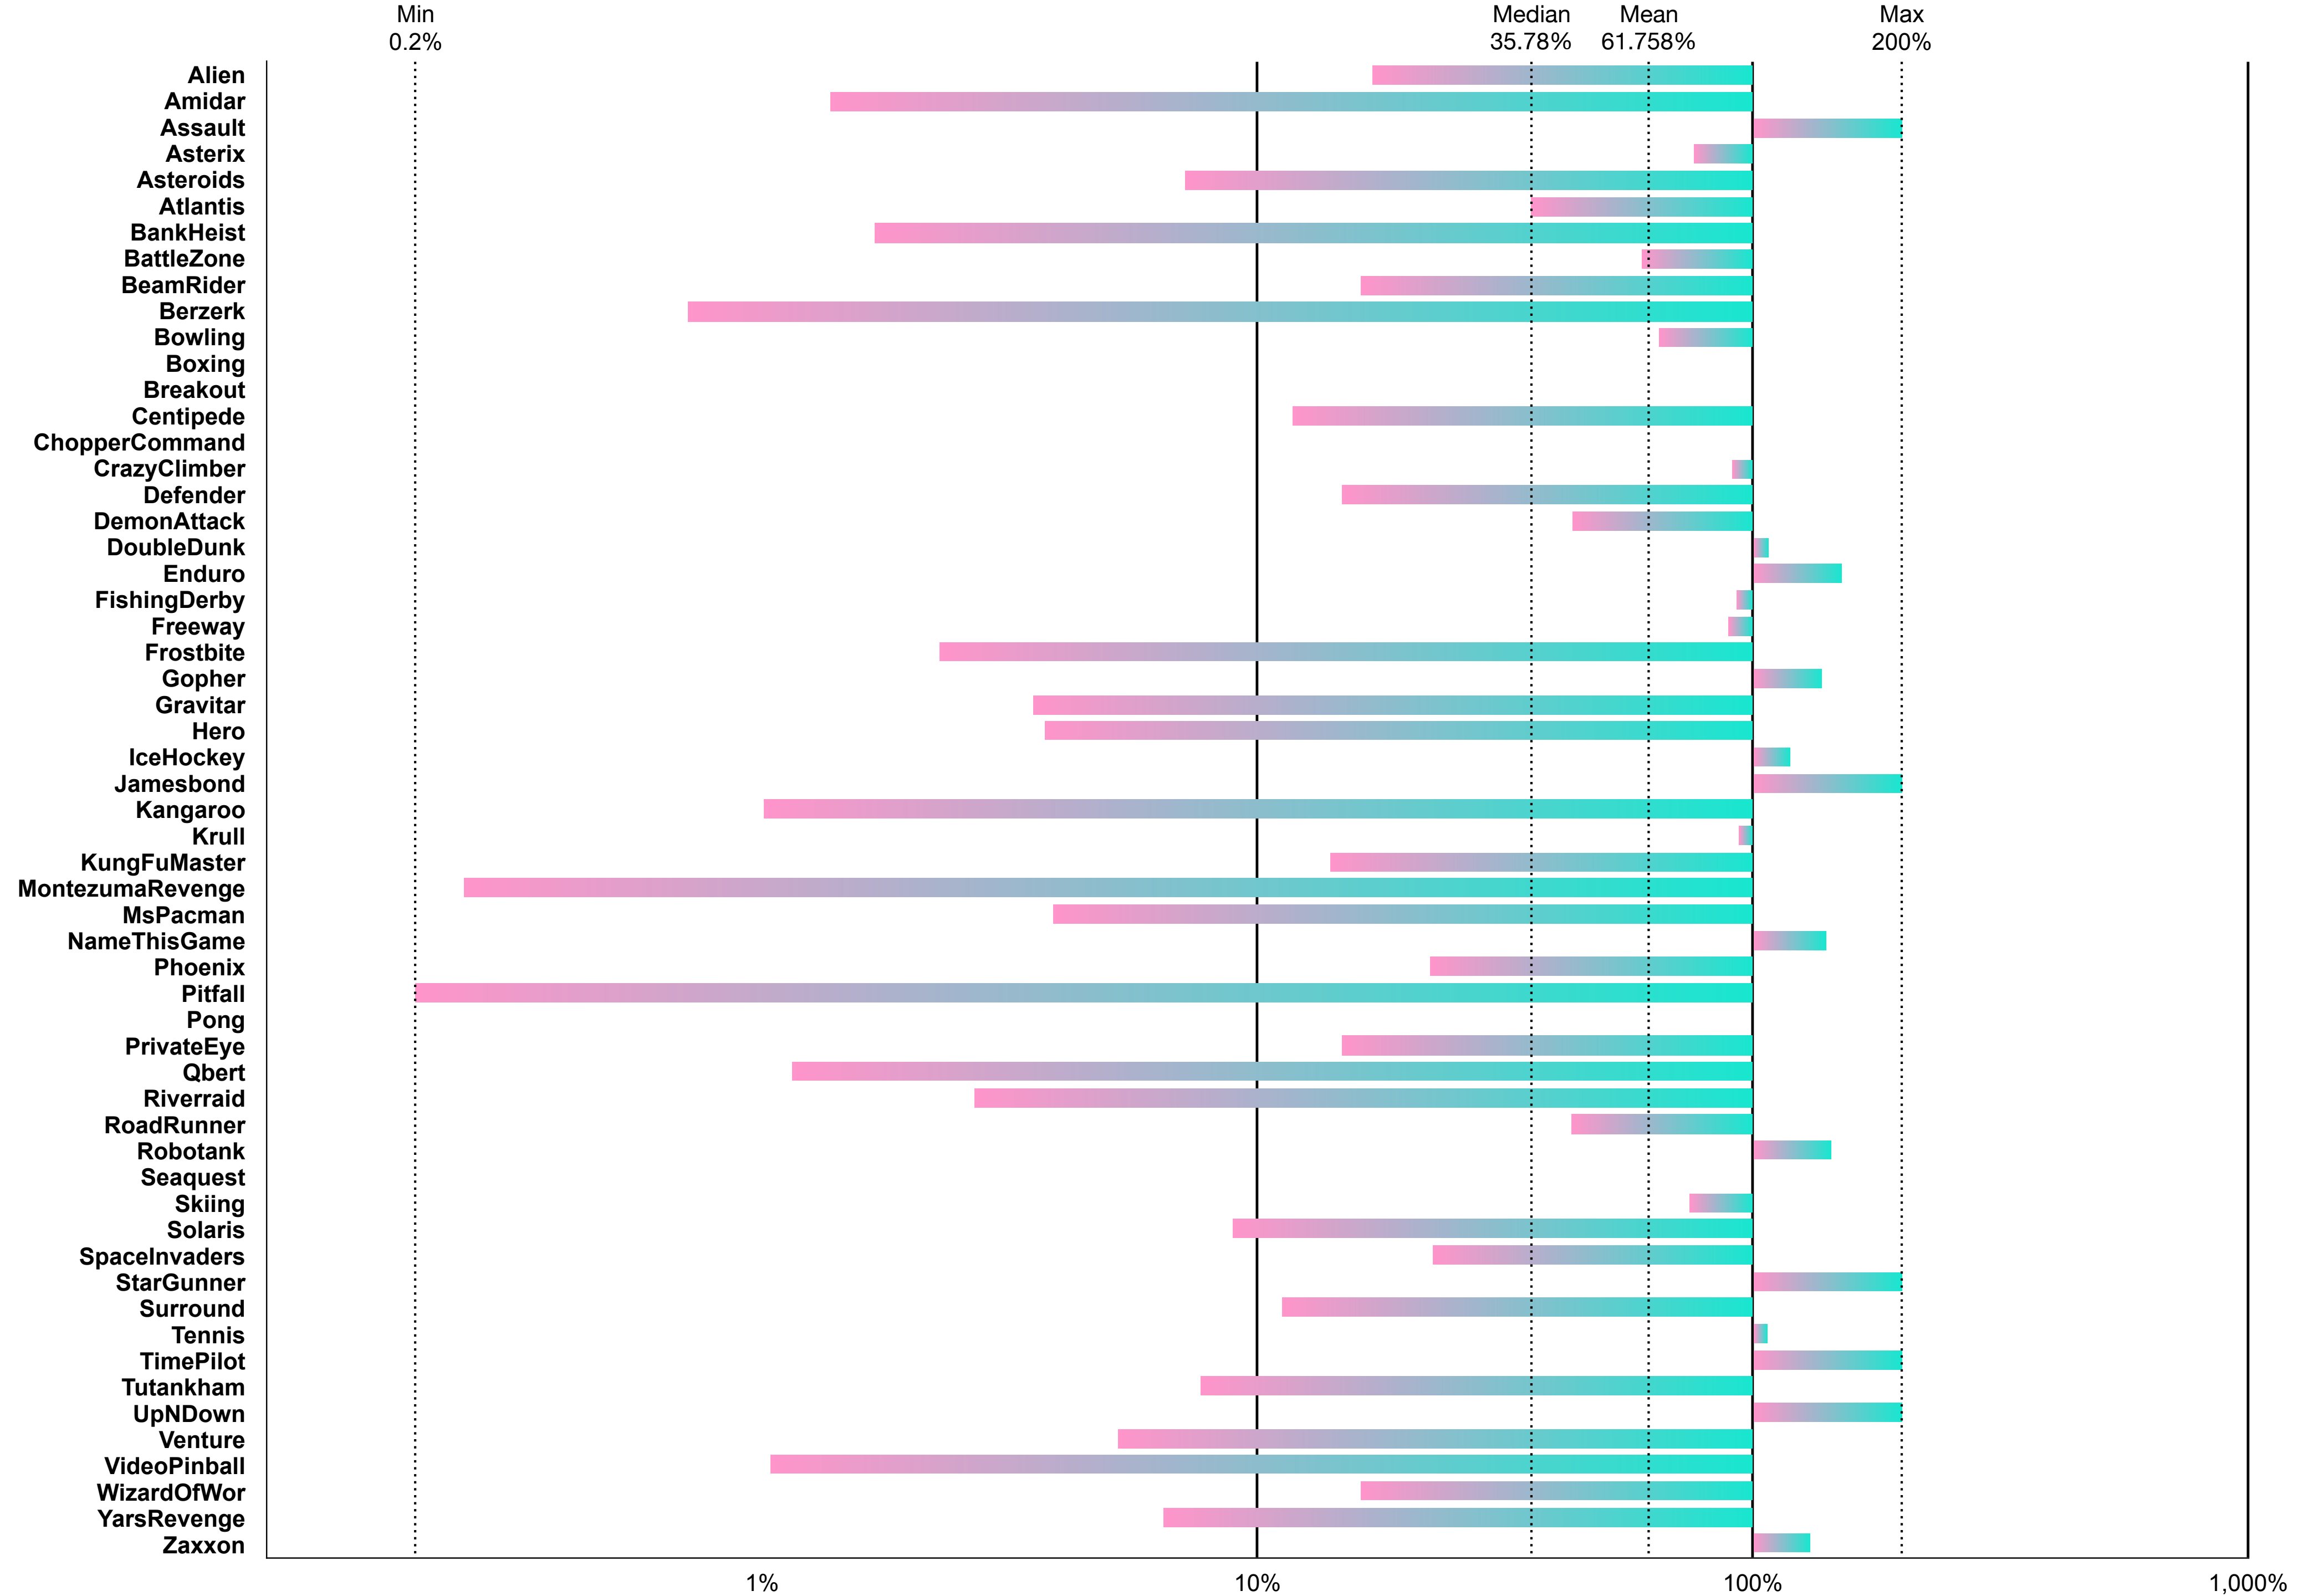

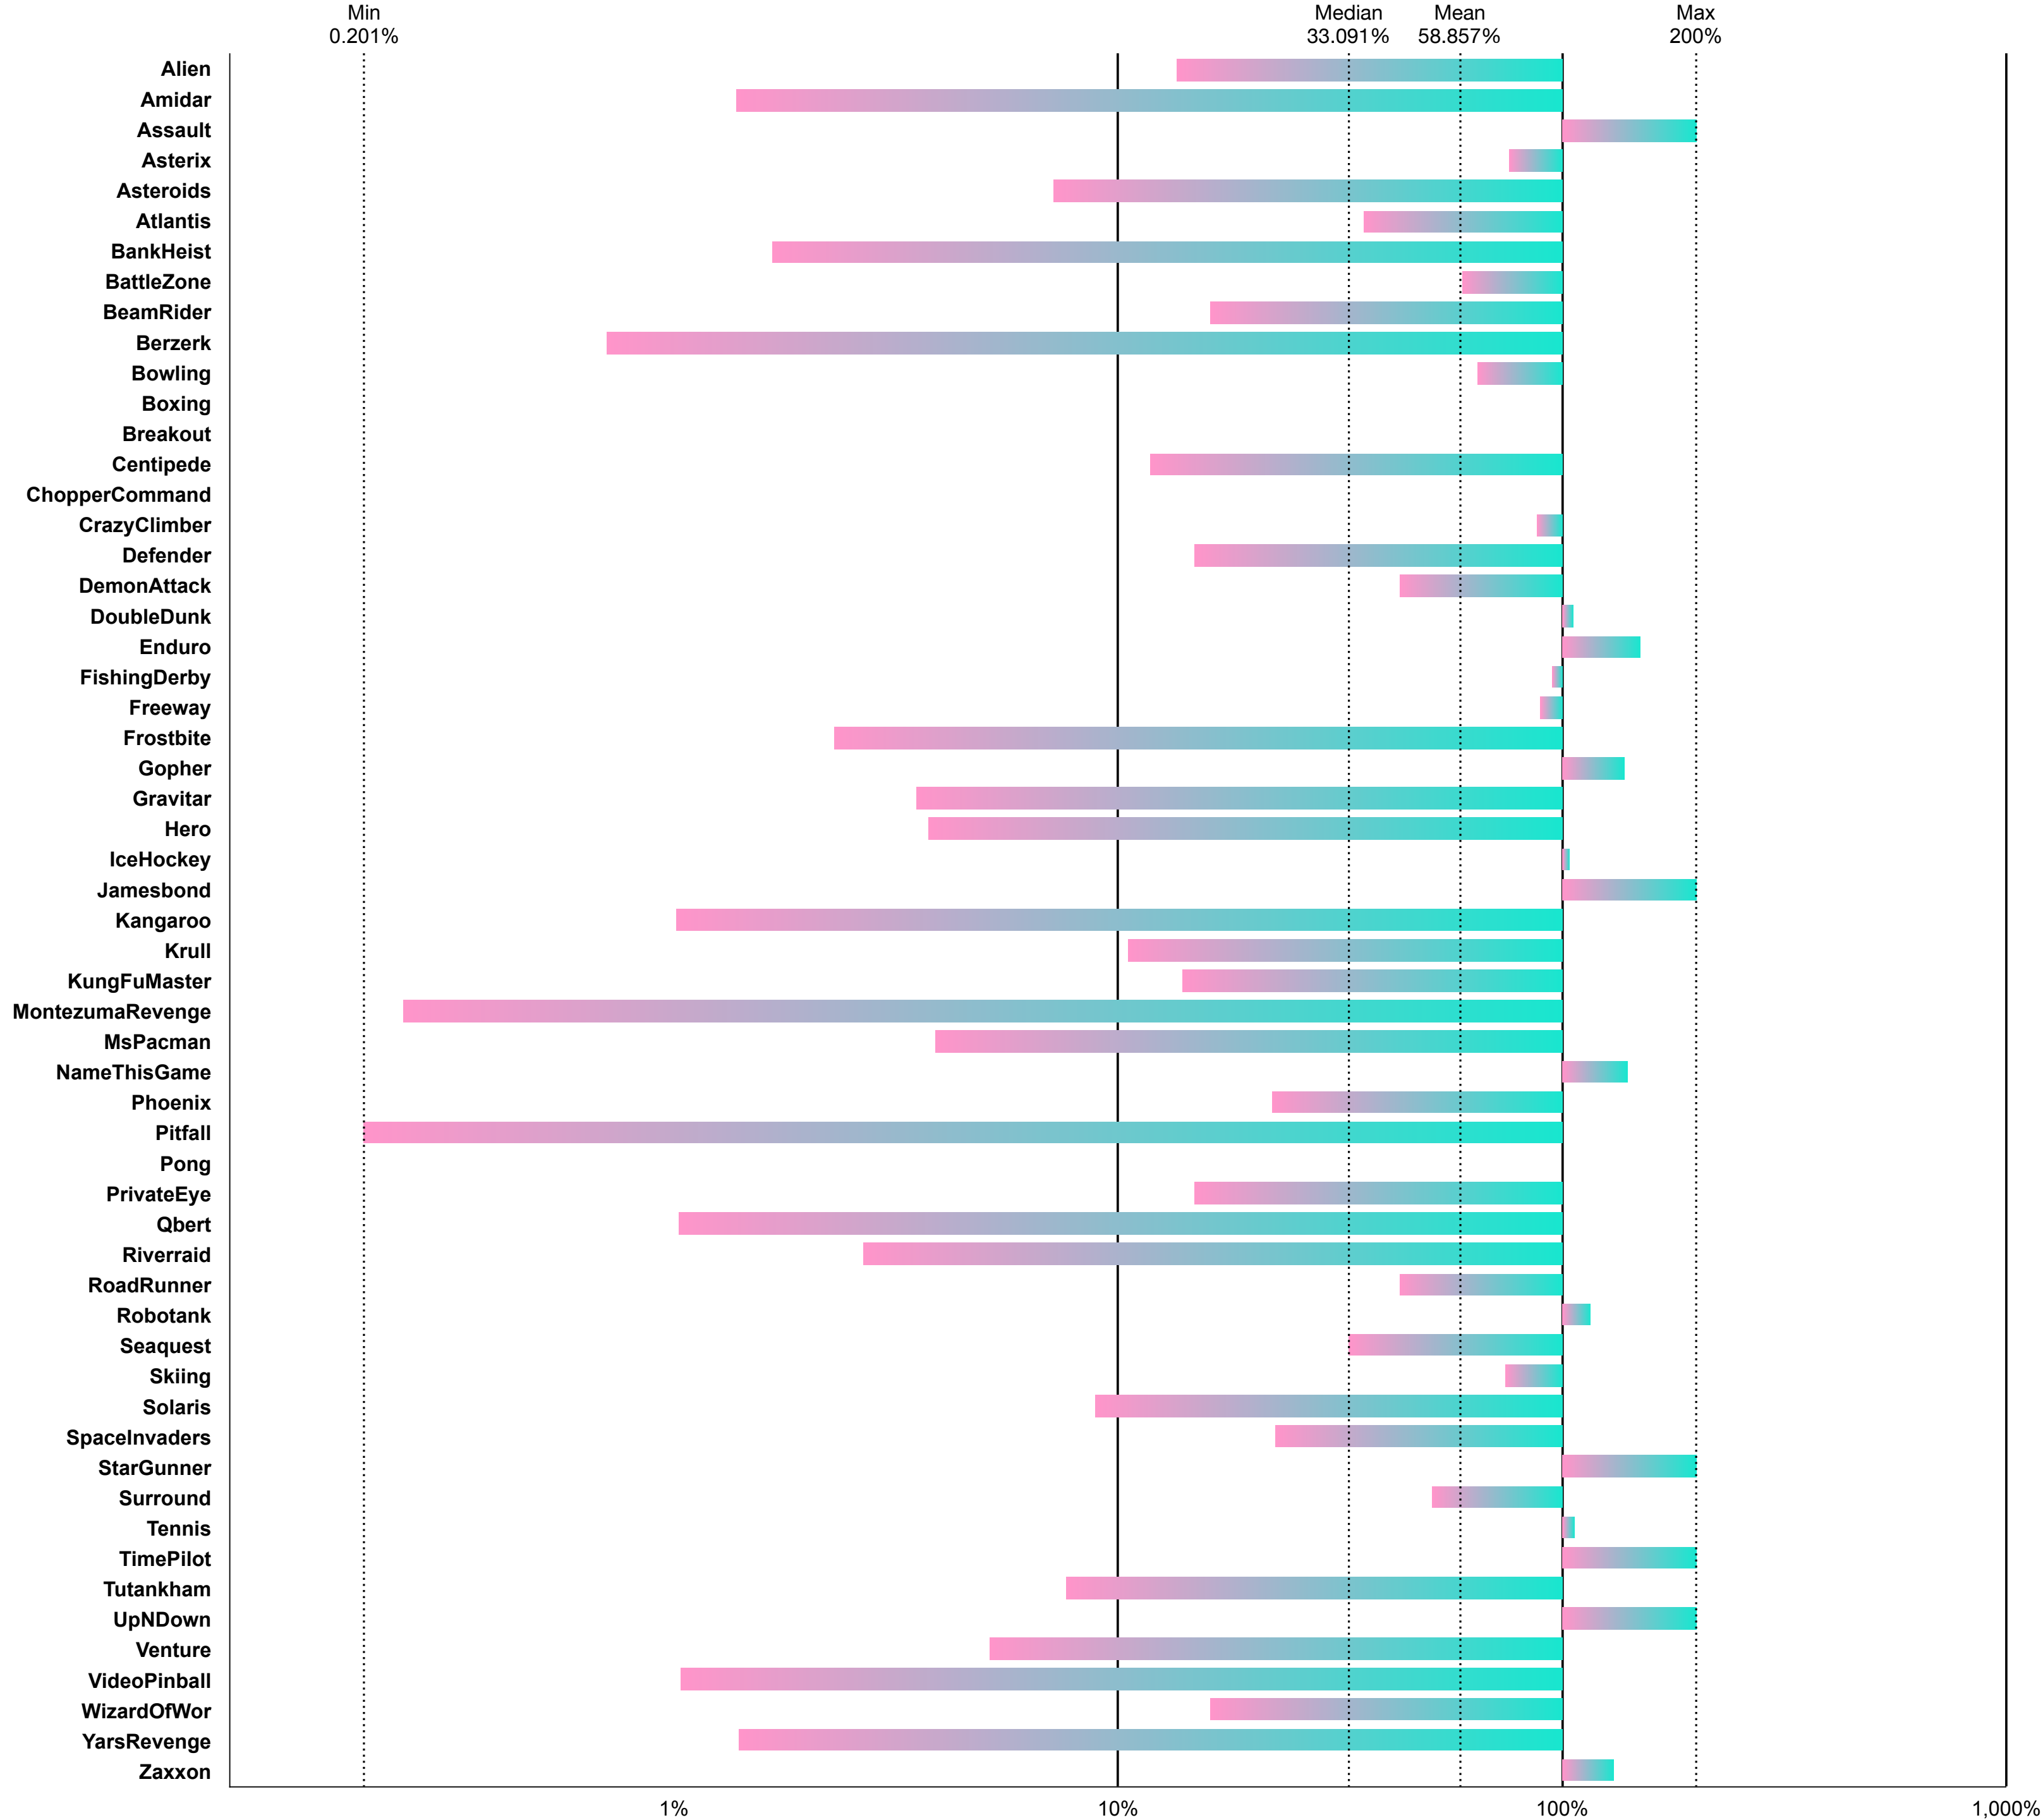

Supplement: Supplementary file 1 [file SABER_capped.pdf]
